# Supplementary material for: Dissipative Tunneling Rates through the Incorporation of First-Principles Electronic Friction in Instanton Rate Theory I: Theory
Source: arXiv:2202.08668 source file (2022-03-09)
Supplement: Supplementary file 1 [file SI-MCTDH.tex]

\section{MCTDH calculations}

\subsection{Flux-side approach}

The thermal rate constant $k_{\beta}$ of the isomerization reaction
$\textrm{A}\rightleftharpoons\textrm{B}$ is traditionally expressed
as the long time limit of a time-dependent ``rate constant'' $k_{\beta}(t)$,
$k_{\beta}=\lim_{t\rightarrow\infty}k_{\beta}(t)$\cite{Yamamoto1960,Miller1983,Miller1998}. The latter involves
the so-called flux-side correlation function $C_{\text{fs}}^{\beta}(t)$
and, in its refined (improved) form\cite{Drozdov2001}, reads as
\begin{equation}
k_{\beta}(t)=\frac{1}{Z_{A}}\frac{C_{\text{fs}}^{\beta}(t)}{P_{A}(0)+\left[P_{A}(0)-1\right]\chi_{\beta}-\left(\frac{1}{Z_{A}}+\frac{1}{Z_{B}}\right)\int_{0}^{t}C_{\text{fs}}^{\beta}(\tau)d\tau}.\label{eq: improved flux-side}
\end{equation}
Here, $h$ is the projection operator that separates the configuration
space of the products from that of the reagents, $Z_{A}$ and $Z_{B}$
are, respectively, the reagent and product partition functions,
\[
Z_{A}=\textrm{Tr}\left(e^{-\beta H}\left(1-h\right)\right)\ \ \ Z_{B}=\textrm{Tr}\left(e^{-\beta H}h\right)
\]
$\chi_{\beta}=Z_{A}/Z_{B}$ is the inverse equilibrium constant of
the reaction, $P_{A}(0)$ is the initial population of the reactants'
well
\[
P_{A}(0)=1-\frac{1}{Z_{A}}\textrm{Tr}\left(e^{-\beta H/2}\left(1-h\right)e^{-\beta H/2}h\right)
\]
and 
\begin{equation}
C_{\text{fs}}^{\beta}(t)=\text{Tr}\left(F_{\beta}h(t)\right)\label{eq:flux-side correlation}
\end{equation}
is the above mentioned flux-side correlation function in its most popular, symmetrized form\cite{Miller1983}. The latter
is the key quantity and requires, besides $h$ above, the Boltzmannized
flux operator
\begin{equation}
F_{\beta}=e^{-\beta H/2}Fe^{-\beta H/2}\ \ \ F=\frac{i}{\hbar}[H,h]\label{eq:Boltzmannized flux operator}
\end{equation}
which is the Boltzmannized version of the Heisenberg time derivative
of $h$ (\emph{i.e.}, the flux operator $F$). In Eq. \ref{eq: improved flux-side}
the long time limit is the true infinite time limit (\emph{i.e.},
the notation $t\rightarrow\infty$ is exact, with no \emph{caveats}),
although in practice the appropriate $t$ is a macroscopically small
time beyond which $k_{\beta}(t)$ approaches a constant value. Since
most often it holds
\[
P_{A}(0)\approx1\ \mathrm{ and} \quad \ \int_{0}^{t_{P}}C_{\text{fs}}(\tau)d\tau\ll\frac{Z_{A}Z_{B}}{Z_{A}+Z_{B}},
\]
the rate takes the form 
\begin{equation}
k_{\beta}\approx\frac{1}{Z_{A}}\lim_{"t\rightarrow\infty"}C_{\text{fs}}(t)\label{eq:flux-side}
\end{equation}
where now the limit needs to be interpreted at the \emph{plateau}
time $t_{P}$ where the correlation function attains a constant value.
Eq. \ref{eq:flux-side} represents the celebrated ``flux-side''
expression of the thermal rate constant. For a derivation of Eq. \ref{eq: improved flux-side} appropriate 
to a condensed-phase environment see Ref. \onlinecite{Craig_JCP_2007}.
%It was originally derived for gas-phase chemical reactions through a 
% rigorous application of scattering theory and it is nowadays applied almost routinely in the condensed phase. 

\subsection{Boltzmann sampling}

We focus here on practical issues that arise when numerically evaluating
the trace expressions of Eq. \ref{eq:flux-side correlation} for a condensed-phase problem involving
many degrees of freedom \cite{Wang2006a,Craig2007}. In particular, we describe the importance sampling scheme introduced by the authors of Ref.s \onlinecite{Wang2006a,Craig2007} to turn the problem into an efficient Monte Carlo sampling of the state space. We shall first describe such 'Monte Carlo wavepacket strategy'
for computing average values of observables and, later, highlight the amendments needed to evaluate the correlation functions.

In the following we assume that $H$ takes the form $H=H_{S}+H_{\text{int}}+H_{B}$
where $H_{S}$ is the system Hamiltonian, $H_{B}$ is a sum of independent
oscillator Hamiltonians and $H_{\text{int}}$ the interaction term
between the system and the bath. Accordingly, for the state space
we have $\mathcal{H}=\mathcal{H}_{S}\otimes\mathcal{H}_{B}$, and
we make use of vectors of the form $\ket{n,N}\equiv\ket{n}\ket{N}$
where $\ket{n}$ is an arbitrary system state and $\ket{N}$ an eigenstate
of the bath, i.e., for $N=\{n_{1}n_{2}..n_{k}...\}$,
\[
H_{B}\ket{N}=E_{N}\ket{N}\ \ \mathrm{and}\quad E_{N}=\sum_{k}\hbar\omega_{k}\left(n_{k}+\frac{1}{2}\right).
\]

\subsubsection{Averages of observables}

The equilibrium average value of an operator $A$ takes the form 
\[
\braket{A}=\frac{1}{Z}\text{Tr}(e^{-\beta H}A)\equiv\frac{1}{Z}\text{Tr}(e^{-\frac{\beta}{2}H}Ae^{-\frac{\beta}{2}H})=\frac{1}{Z}\sum_{n,N}\braket{\Psi_{n,N}^{\beta}|A|\Psi_{n,N}^{\beta}}
\]
where $\ket{\Psi_{n,N}^{\beta}}=e^{-\frac{\beta}{2}H}\ket{n,N}$.
This equation is best re-written in terms of \emph{normalized} vectors
$\ket{\Phi_{n,N}^{\beta}}$, which are those directly available from
the MCTDH package upon imaginary-time evolution. Clearly, for a solution
of the Bloch equation
\[
-\frac{\partial\ket{\Psi_{\beta}}}{\partial\beta}=H\ket{\Psi}\ \ \ \ket{\Psi_{\beta=0}}=\ket{\Psi_{0}}
\]
given its squared norm $p(\beta)=\braket{\Psi_{\beta}|\Psi_{\beta}}$
and the energy expectation $\epsilon(\beta)=\braket{\Psi_{\beta}|H|\Psi_{\beta}}/p(\beta)$,
we have $\frac{\partial p}{\partial\beta}(\beta)=-2\epsilon(\beta)p(\beta)$,
hence $p\left(\beta\right)=e^{-2\int_{0}^{\beta}\epsilon(\tau)d\tau}$
and $\ket{\Psi_{\beta}}=e^{-\int_{0}^{\beta}\epsilon(\tau)d\tau}\ket{\Phi_{\beta}}$.
Thus, 
\begin{align*}
\braket{A} & =\frac{1}{Z}\sum_{n,N}p_{n,N}\left(\frac{\beta}{2}\right)\braket{\Phi_{n,N}^{\beta}|A|\Phi_{n,N}^{\beta}}\\
 & =\frac{Z_{0}}{Z}\sum_{N}\frac{e^{-\beta E_{N}}}{Z_{0}}\sum_{n}W_{n,N}(\beta)\braket{A}_{n,N}^{\beta}
\end{align*}
where $Z_{0}$ is the partition function of the uncoupled bath, $\braket{A}_{n,N}^{\beta}=\braket{\Phi_{n,N}^{\beta}|A|\Phi_{n,N}^{\beta}}$
are expectation values and
\begin{equation}
W_{n,N}(\beta)=e^{+\beta E_{N}}e^{-2\int_{0}^{\beta/2}\epsilon_{n,N}(\tau)d\tau}\label{eq:thermal weight factors}
\end{equation}
are thermal factors determined 
by the average energy  $\epsilon_{n,N}(\tau)$ of the state $\ket{\Phi_{n,N}^{\tau}}$ during
the imaginary-time evolution. The ensemble-average takes thus the
form of a Boltzmann-weighted sum of terms which can be efficiently
evaluated \emph{via} Monte Carlo sampling,
\begin{equation}
\braket{A}=\frac{Z_{0}}{Z}\sum_{n}\llangle W_{n,N}(\beta)\braket{A}_{n,N}^{\beta}\rrangle\label{eq:Monte-Carlo sampling <A>}
\end{equation}
where the double bracket denotes the Boltzmann average (and $N$ is
the corresponding random variable). This expression can be further
rewritten upon noticing that  $Z=Z_{0}\sum_{n}\llangle\ W_{n,N}(\beta)\ \rrangle$
(as it follows from Eq. \ref{eq:Monte-Carlo sampling <A>} upon setting
$A=1$), hence
\begin{equation}
\braket{A}=\frac{\sum_{n}\llangle\ W_{n,N}(\beta)\braket{A}_{n,N}^{\beta}\rrangle}{\sum_{n}\llangle\ W_{n,N}(\beta) \rrangle}\label{eq:A expectation Monte-Carlo}
\end{equation}
which requires just one sampling. 

\begin{figure}
\begin{centering}
\includegraphics[width=0.9\textwidth]{Figs/sampling}
\par\end{centering}
\caption{\label{fig:Sampling-of-the bath}Sampling of the bath (results for
a typical bath containing $F=50$ oscillators). Left: individual energy
of the bath states $\ket{N_{I}}$ sampled at different temperatures
($N_{\text{MC}}=128$ realizations for clarity), along with the theoretical
mean energy $\braket{E}$ (yellow) and $\braket{E}\pm\Delta E$ (cyan),
where $\Delta E^{2}$ is the energy variance. Right: average occupation
numbers $n_{k}$ obtained for $N_{\text{MC}}=128,256$ realization,
compared with the exact results (dashed lines).}
\end{figure}
In practice, given a basis of $\mathcal{H}_{S}$ a number of bath
configurations $\ket{N_{i}}$ are generated from the Boltzmann distribution
and the vectors $\ket{n,N_{i}}$ are propagated in imaginary-time
to compute the expectation values and the thermal factors. Sampling
can be performed independently for each bath oscillator, using the
known cumulative distributions $P_{\nu}=\sum_{k=0}^{\nu}\rho_{k}$ (where
$\rho_{k}$ are the Boltzmann probabilities) of a harmonic oscillator
with frequency $\omega$,
\[
P_{\nu}=1-e^{-\beta\hbar\omega(\nu+1)}.
\]
That is, $\nu_{i}=\text{int}(-\ln(\xi_{i}/\beta\hbar\omega))$, for
$\xi_{i}$ random in $[0,1]$, gives a set of quantum numbers $\nu_{i}$
Boltzmann distributed. Thus, besides bookkeeping issues, the procedure
is entirely straightforward and generates vectors $\ket{N_{I}}\equiv\ket{n_{i_{1}}}\ket{n_{i_{2}}}..\ket{n_{i_{k}}}..\ket{n_{i_{F}}}$
where $I=(i_{1}i_{2}..i_{k}..i_{F})$ and $F$ is the number of bath
degrees of freedom. Fig. \ref{fig:Sampling-of-the bath} illustrates
typical results of such sampling for the case considered in the main
text, which used $F=50$ harmonic oscillators with frequencies 
\[
\omega_{k}=-\omega_{c}\ln\left(\frac{k}{F+1}\right)
\]
where $\omega_{c}$ is a cutoff frequency. This is a widely used discretization
of the Ohmic bath with exponential cutoff, $J(\omega)=m\gamma\omega e^{-\omega/\omega_{c}}$,
provided the couplings $c_{k}$ with the system coordinate are set
according to 
\[
c_{k}=\omega_{k}\sqrt{\frac{2}{\pi}\frac{m\gamma\omega_{c}}{F+1}M}
\]
where $m$ and $M$ are, respectively, the system and the oscillators
mass, and $\gamma$ is the damping coefficient ($\gamma=\tilde{\eta}_0/m$, with $\tilde{\eta}_0$ being the static friction coefficient as defined in the main text.). Here, the cutoff frequency
was set to $\omega_{c}=500$ cm$^{-1}$. 

Importantly, we notice that the reagent partition function takes a form similar to the total partition function 
\begin{equation}
Z_{A}=Z_{0}\sum_{n}\llangle\ W_{n,N}(\beta)\braket{h_{A}}_{n,N}^{\beta}\ \rrangle\label{eq:reagent partition function Monte Carlo}
\end{equation}
but now the system states are better chosen to closely resemble ``the
reagent states'' since, in practice, a quickly convergent sum over
$n$ is highly desirable. In our implementation they are eigenstates
of a fictitious Hamiltonian that describes reagents only, \emph{i.e.
}the states $\ket{n}$ are chosen to be eigenstates of $\tilde{H}_{S}=\frac{p^{2}}{2m}+\tilde{v}$
where $\tilde{v}$ is a modified potential with the ``reaction channel
artificially closed''. This choice improves much the Monte Carlo
convergence and, in practice, requires 1-2 system states (depending
on the temperature) to obtain a numerically converged value of the
reagent partition function. Notice further that the convergence depends
also on other numerical parameters. For instance, a grid for the bath
oscillations that is ``centered'' around the classical equilibrium
position (the reagent minimum of the potential) is much more efficient
that an ``unbiased'' grid (like the one appropriate for the flux
evaluation). That is, for the typical Hamiltonian
\[
H=H_{S}+\sum_{k}\left[\frac{p_{k}^{2}}{2M}+\frac{M\omega_{k}^{2}}{2}\left(x_{k}-\frac{c_{k}s}{M\omega_{k}^{2}}\right)^{2}\right]
\]
the center of the grid for the $k^{\text{th}}$ harmonic oscillator
is better placed at 
\[
x^{\ominus}=\frac{c_{k}}{M\omega_{k}^{2}}s_{\text{min}}
\]
where $s_{\text{min}}$ is the value of the system coordinate at the
bottom of the reagent well. 

\subsubsection{Flux-side correlation}

The standard flux-side correlation $C_{\text{fs}}^{\beta}\equiv\text{Tr}(e^{-\frac{\beta}{2}H}Fe^{-\frac{\beta}{2}H}h(t))$
can be evaluated similarly to the expectation values considered above
by introducing the spectral representation of $F=\sum_{u}u\ket{u}\bra{u}$
and re-writing the trace as a sum over states
\[
C_{\text{fs}}^{\beta}(t)=\sum_{u}\sum_{N}u\braket{uN|h(\tau)|uN}
\]
where the expectation of the operator $h(\text{\ensuremath{\tau}})=e^{\frac{i}{\hbar}H\tau^{*}}he^{-\frac{i}{\hbar}H\tau}$
(with $\tau=t-i\frac{\hbar\beta}{2}$) requires both the imaginary
and the real time evolution. This general procedure is, however, numerically
inconvenient since $F$ (albeit \emph{system-only}) has many contributing
eigenstates, thereby making the sum over $u$ rather long\footnote{Notice that the total number of wavepackets is given by $M\times N_{\text{MC}}$,
where $M$ is number of contributing system states and $N_{\text{MC}}$
the size of the Monte Carlo ensemble for the bath, typically $N_{\text{MC}}=128-256$.}. Fortunately, at least for the case we are interested in, there is
a way out of this ``dimensionality'' problem: the \emph{Boltzmannized}
flux operator is intrinsically of low-rank, that is it reads as
\[
F_{\beta}^{S}=e^{-\frac{\beta}{2}H_{S}}Fe^{-\frac{\beta}{2}H_{S}}=\sum_{\nu}\nu(\beta)\ket{\nu_{\beta}}\bra{\nu_{\beta}}
\]
where only few values of $\nu(\beta)$'s are significant (in fact
just two, related to each other by time inversion, if the temperature
is low enough, as it easily follows by the two-state approximation
of the dynamics)\footnote{Notice that $F$ here is a \emph{system-only} operator and that the
above expression is of low rank only in the space of system states
$\mathcal{H}_{S}$: when the same operator is considered in the whole
space $\mathcal{H}$ each eigenflux space becomes highly degenerate.}. Fig. \ref{fig:Boltmannized-flux-eigenstates} illustrates the typical
behavior of the most important flux eigenstates at varying temperatures,
and their relation to the energy eigenstates. 
\begin{figure}
\begin{centering}
\includegraphics[width=1\textwidth]{Figs/eigen2}
\par\end{centering}
\caption{\label{fig:Boltmannized-flux-eigenstates}Boltmannized flux eigenstates
$\ket{\nu_{\beta}}$ for a symmetric double well potential (black
curves). Left: the two lowest-lying energy eigenstates forming the
ground-state tunneling-split doublet. Right: the absolute value of
the Boltzmannized-flux eigenfunction with the largest positive eigenvalue,
as obtained at the indicated temperatures (vertically shifted for
clarity). $a_0$ refers to the Bohr radius.}
\end{figure}
 To exploit the above property, following Craig \emph{et al. } \cite{Craig_JCP_2007}, we
write
\begin{align*}
F & =e^{+\frac{\beta}{2}H_{S}}F_{\beta}^{S}e^{+\frac{\beta}{2}H_{S}}=\sum_{\nu}\nu(\beta)e^{+\frac{\beta}{2}H_{S}}\ket{\nu_{\beta}}\bra{\nu_{\beta}}e^{+\frac{\beta}{2}H_{S}}\\
 & \equiv\sum_{\nu}w_{\nu}(\beta)\ket{\bar{\nu}_{\beta}}\bra{\bar{\nu}_{\beta}}
\end{align*}
where $\ket{\bar{\nu}_{\beta}}$ are normalized, imaginary-time backward-propagated
flux eigenvectors, 
\[
\ket{\bar{\nu}_{\beta}}=\frac{1}{\sqrt{\braket{\nu_{\beta}|e^{\beta H_{S}}|\nu_{\beta}}}}e^{\beta H_{S}/2}\ket{\nu}
\]
and $w_{\nu}(\beta)=\nu(\beta)\braket{\nu_{\beta}|e^{\beta H_{S}}|\nu_{\beta}}$
are flux-weights. The $\ket{\bar{\nu}_{\beta}}$'s are non-orthogonal, yet rather useful since they provide a compact representation of the flux operator. With these definitions, we have
\begin{align*}
C_{\text{fs}}^{\beta} & =\sum_{\nu}\text{Tr}\left(e^{-\beta H/2}\ket{\bar{\nu}_{\beta}}\bra{\bar{\nu}_{\beta}}e^{-\beta H/2}h(t)\right)w_{\nu}(\beta)\\
 & \equiv\sum_{\nu}\sum_{N}w_{\nu}(\beta)\braket{\bar{\nu}_{\beta}N|e^{-\beta H/2}h(t)e^{-\beta H/2}|\bar{\nu}_{\beta}N}
\end{align*}
and everything proceeds as above. Specifically, introducing the normalized
vectors
\[
\ket{\Phi_{\nu,N}^{\beta}}=\frac{1}{\sqrt{p_{\nu N}(\beta)}}e^{-\beta H/2}\ket{\bar{\nu}_{S}N}\ , \quad\ p_{\nu N}(\beta)=e^{-2\int_{0}^{\beta/2}\epsilon_{\nu N}(\tau)d\tau},
\]
their real-time evolutions 
\[
\ket{\Phi_{\nu,N}^{\beta}(t)}=e^{-\frac{i}{\hbar}Ht}\ket{\Phi_{\nu,N}^{\beta}}
\]
and the expectation $\braket{h(t)}_{\nu N}^{\beta}=\braket{\Phi_{\nu,N}^{\beta}(t)|h|\Phi_{\nu,N}^{\beta}(t)}$
we write
\[
C_{\text{fs}}^{\beta}=Z_{0}\sum_{N}\frac{e^{-\beta E_{N}}}{Z_{0}}\sum_{\nu}w_{\nu}(\beta)W_{\nu N}(\beta)\braket{h(t)}_{\nu N}^{\beta},
\]
where $W_{\nu N}(\beta)=p_{\nu N}(\beta)e^{\beta E_{N}}$ are thermal
factors (Eq. \ref{eq:thermal weight factors}) and $w_{\nu}(\beta)$
are (thermal) flux weights. Equivalently, 
\begin{equation}
C_{\text{fs}}(t)=Z_{0}\sum_{\nu}\llangle\ w_{\nu}(\beta)W_{\nu N}(\beta)\braket{h(t)}_{\nu N}^{\beta}\rrangle\label{eq:flux-side correlation Monte Carlo}
\end{equation}
is the working expression involving 
\begin{itemize}
\item [{\emph{(i-a)}}] a ``system'' preparation to define the appropriate
system states $\ket{\bar{\nu}_{\beta}}$, 
\item [{\emph{(i-b)}}] a Monte Carlo sampling of the (uncoupled) bath state,
which delivers bath states $\ket{N}$, 
\item [{\emph{(ii)}}] a relaxation dynamics with the full Hamiltonian
$H$ for each state $\ket{\bar{\nu}_{\beta}N}$ 
\item [{\emph{(iii)}}] a real time dynamics with the same Hamiltonian
on the relaxed states obtained in \emph{(ii)}. 
\end{itemize}
When combined with the calculation of the reagent partition function,
Eq. \ref{eq:reagent partition function Monte Carlo}, this recipe
gives the thermal rate constant of Eq. \ref{eq:flux-side} or, with
minor additional effort, the one defined by Eq. \ref{eq: improved flux-side}.

In closing this section it is worth noticing that the manipulations
above with the Boltzmann operator are well defined when the Hamiltonian
operator $H_{S}$ is bound\footnote{When a maximum eigenvalue exists the Boltzmann operator is non-singular.}
but some regularization is needed when --- as it is often the case in
realistic problems --- the spectrum of $H_{S}$ is unbound. This is particularly important for numerical applications because
the presence of high-lying energy eigenstates makes $\exp\left(-\beta H_{S}\right)$
nearly singular and $\exp\left(+\beta H_{S}\right)$ numerically unstable,
increasingly so when reducing the temperature ($\beta\rightarrow\infty$).
Fortunately, such high-lying energy eigenstates should not play any
role in the dynamics (particularly at the low temperatures where a
quantum description is required) and the simple regularization of
replacing $H_{S}$ with its projection $\bar{H}_{S}$ on a low-lying
energy eigenspace suffices. Specifically, defining $P_{n}$ the projection
onto the first (lowest lying) $n$ eigenstates of $H_{S}$ one defines
$\bar{H}_{S}=P_{n}H_{S}P_{n}$ and uses it in place of $H_{S}$ in
some of the expressions above. This is entirely legitimate since the
aim is just to re-write $F$ in a suitable way, but of course one
must ensure that $\bar{H}_{S}$ closely resembles $H_{S}$ for the
expansion to be compact. In practice, then, one uses $H_{S}$ to define
the Boltzmannized flux and diagonalize it, and then switches to $\bar{H}_{S}$
when propagating backward in imaginary time, making sure that the
``error'' is kept below a desired threshold\footnote{The reliability of such regularization can be measured by the difference
in the (differently) Boltzmannized flux eigenvalues and by two kinds
of errors in the flux eigenstates: there exists a \emph{truncation}
error (the distance between the eigenvectors of the differently Boltzmannized
operators) and a \emph{propagation} error (defined by back-propagating
with the ``projected version'' of the Boltzmann operator followed
by propagation with the true Boltzmann operator). The latter two behave
oppositely when varying $n$ since the truncation error determines
the quality of the projected Hamiltonian and the propagation error
reflects the above mentioned numerical instability.}$^{,}$\footnote{There is no need for $H_{S}$ to be the same ``system'' Hamiltonian
appearing in the total Hamiltonian, and one can set it at his own
convenience. After all the flux operator $F$ does \emph{not} depend
on the potential. }. 

\subsection{ML-MCTDH wavefunction and calculation setup}

\begin{figure}
\begin{centering}
\includegraphics[angle=90,height=0.8\textheight]{Figs/mltree}
\par\end{centering}
\caption{\label{fig:ML-tree}Adopted tree structure for the ML-MCTDH wavefunction. Each circle denotes a MCTDH-like expansion in the tree, along with its modes (the arms) and the number of the single particle functions used in the expansion (the numbers on the arms). Squares denote the bottom layers where modes reduce to physical degrees of freedom and the numbers represent the size of the primitive grids. Here $x$ is the system coordinate and the $q_k$'s are bath coordinates.}
\end{figure}
Fig. \ref{fig:ML-tree} shows the tree structure defining the ML-MCTDH wavefunction.
It was obtained after extensive testing, and found to accurately reproduce
previous ML-MCTDH and PI results, at both high and low temperatures at varying coupling strengths, ranging from the weak to the strong coupling limits. The number of logical modes
used in each layer was kept small ($2-3$) and each of them was described
with several single-particle functions ($12-6$). Only in the bottom
layer, depending on the size of the primitive grids, the bath degrees
of freedom (the ``$q_{k}$''s in Fig. \ref{fig:ML-tree}, sorted
in order of increasing frequency) were grouped in $3-4$ dimensional
single-particles. The system mode (the ``$x$'' in Fig. \ref{fig:ML-tree})
is located in the group of bath modes with comparable frequency, although
described separately from the bath modes and with the help of a large
number of SPFs. As for the primitive grids we used Harmonic Oscillator - Discrete Value Representation (HO-DVR) grids for
each bath degrees of freedom, which amounts to introduce a phonon
basis of the same size for the corresponding mode. The grids for the low
frequency modes used several tens of points (as indicated in Fig.
\ref{fig:ML-tree}), and were extended if necessary to accommodate each realization sampled from the canonical ensemble of the bath. The grids for the high-frequency
modes, on the other hand, used much fewer grid points since they were barely excited during
the dynamics. The system degree of freedom was described with a uniformly
spaced grid, a Fast Fourier Transform - Discrete Value Representation (FFT-DVR), using 512 grid points in the range $x\in[-4,4]\ a_{0}$ (with $a_0$ referring to the Bohr radius). 

\begin{figure}
\begin{centering}
\includegraphics[width=0.95\columnwidth]{Figs/thermal_factors}
\par\end{centering}
\caption{\label{fig:Thermal factors}Behavior of the thermal factors otained
in thermalization step. Left: individual realizations, with their
average and root mean square given as red curve with error bars. Right:
root mean square for different temperatures, as a function of the
coupling strength.}

\end{figure}
\begin{figure}
\begin{centering}
\includegraphics[width=0.95\columnwidth]{Figs/flux-side-LC}
\par\end{centering}
\caption{\label{fig:Illustrative-examples-of-Cfs}Illustrative examples showing
the behavior of the flux-side correlation function  at $T = 90$ K (top row) and $T=50$ K (bottom row),
for very small and large coupling strength, $\gamma/\omega_b=0.01$ and $0.95$, respectively for the left and right panels. Gray (green) area shows the spread (statistical error) calculated as the root-mean-square deviation of $x_N$ (root-mean-square deviation of $x_N$ over square-root of number of realizations).}

\end{figure}
The MCTDH equations of motion were integrated with the Variable Mean
Field scheme, using a variable step-size $8^{\text{th}}$-order Runge-Kutta
integrator for both the amplitude coefficients and the single-particle
wavefunctions, and a small accuracy parameter ($10^{-8}$). The propagation
time was set differently according to the coupling strength, in order
to guarantee that the computed flux-side correlation functions attained
a constant limiting value (which occurs at increasingly longer times
when decreasing friction). Similarly, the number of realization was
chosen differently depending on the considered temperature and coupling
strength, the higher $T$ and/or $\gamma$ the larger the number of
realizations used. Fig. \ref{fig:Thermal factors} shows the behavior
of the thermal factors of Eq. \ref{eq:thermal weight factors} as
computed in the ``equilibration step'' (step ii above), which are
the weights with which the individual realizations of the bath enter
into the flux-side correlation function expression of Eq. \ref{eq:flux-side correlation Monte Carlo}
(for a given flux state). Their logarithms are within $0-2$ over
a wide range of coupling strengths, meaning roughly that each realization
has a weight in a two-order-of-magnitude wide interval at most. Fig. \ref{fig:Illustrative-examples-of-Cfs},
on the other hand, displays some illustrative examples of the evolution
of the correlation functions, along with the spread of the contributing
terms in the sum of Eq. \ref{eq:flux-side correlation Monte Carlo}. More specifically, the latter was obtained by grouping results from opposite flux eigenvalues, and rewriting Eq. \ref{eq:flux-side correlation Monte Carlo} as an average of individual contributions $x_N =\sum_\nu W_{\nu N} |w_\nu (\beta)| \left[\braket{h}_{+|\nu|, N}-\braket{h}_{-|\nu|, N}\right]$ with a spread given by the root-mean-square deviation of the  $x_N$'s. Hence, provided bath sampling is sufficiently extended, it measures the intrinsic variability of the reaction probability across the thermal equilibrium state.
